# Supplementary material for: Secondary electron interference from trigonal warping in clean carbon nanotubes
Source: arXiv:1602.03866 ancillary file (2016-08-22)
Supplement: Supplementary file 1 [file supplement.pdf]

# Secondary electron interference from trigonal warping in clean carbon nanotubes

## Supplementary Material

A. Dirnaichner,<sup>1,2</sup> M. del Valle,<sup>2</sup> K. J. G. Götz,<sup>1</sup> F. J. Schupp,<sup>1</sup>  
N. Paradiso,<sup>1</sup> M. Grifoni,<sup>2</sup> Ch. Strunk,<sup>1</sup> and A. K. Hüttel<sup>1,\*</sup>

<sup>1</sup>*Institute for Experimental and Applied Physics,  
University of Regensburg, 93040 Regensburg, Germany*

<sup>2</sup>*Institute for Theoretical Physics, University of Regensburg, 93040 Regensburg, Germany*

(Dated: August 22, 2016)

### CONTENTS

|                                                                                  |    |
|----------------------------------------------------------------------------------|----|
| I. Sample fabrication and experimental setup                                     | 1  |
| II. Fourier analysis and estimation of the average length of the electronic path | 1  |
| III. Transfer matrix approach                                                    | 3  |
| IV. Tight-binding calculations                                                   | 4  |
| V. Estimate of the error in determining the chiral angle                         | 8  |
| References                                                                       | 10 |

### I. SAMPLE FABRICATION AND EXPERIMENTAL SETUP

As electrode material, a 10/40 nm Ti/Pt bilayer is patterned on top of a degenerately doped Si substrate with a 500 nm thick insulating capping layer, see Fig. S1. In order to avoid contamination of the CNT, we grow the carbon nanotube as a last fabrication step across the contact electrodes separated by a  $1.2\,\mu\text{m}$  trench.<sup>1</sup> The identification of a promising device is done solely via room temperature transport measurements using a probe station. This is necessary to avoid contamination of the nanotube. The transport measurements presented in the main text, Fig. 1, were recorded at a base temperature of 15 mK in a  $^3\text{He}/^4\text{He}$  dilution refrigerator. All data shown in the main text is recorded in a standard DC measurement setup, see schematics in Fig. S1. Voltage sources are connected to the source contact and to the doped substrate while the drain contact is grounded. The current is measured at the drain contact using a current-voltage converter. The conductance data is obtained by numerical derivation.

### II. FOURIER ANALYSIS AND ESTIMATION OF THE AVERAGE LENGTH OF THE ELECTRONIC PATH

Within this section we analyze some consequences of the application of Eq. (1) of the main text. Eq. (1) describes the transmission originating from two independent channels  $a$  and  $b$ , i.e., channels with no scattering into each other. Therefore it strictly applies to *armchair*, *zigzag* and *zigzag-like* CNTs. However, the following analysis provides an insight on the suppression of higher harmonics in *armchair-like* CNTs as well.

Let us have a closer look at the transmission formula, Eq. (1) of the main text. We focus on the case of armchair CNTs, where the phase relation can be written as  $\phi_j(V_g, L) = 2k_j(V_g)L$ , where  $k_j = k_{j,l} = k_{j,r}$  for both channels  $j \in \{a, b\}$ . The transmission then becomes

$$\mathcal{T}(V_g) = 2 \sum_{j \in \{a, b\}} T(k_j) = 2 \sum_{j \in \{a, b\}} \frac{|t_1|^2 |t_2|^2}{(1 - |r_1| |r_2|)^2 + 4 |r_1| |r_2| \sin^2[k_j L]}. \quad (\text{S1})$$

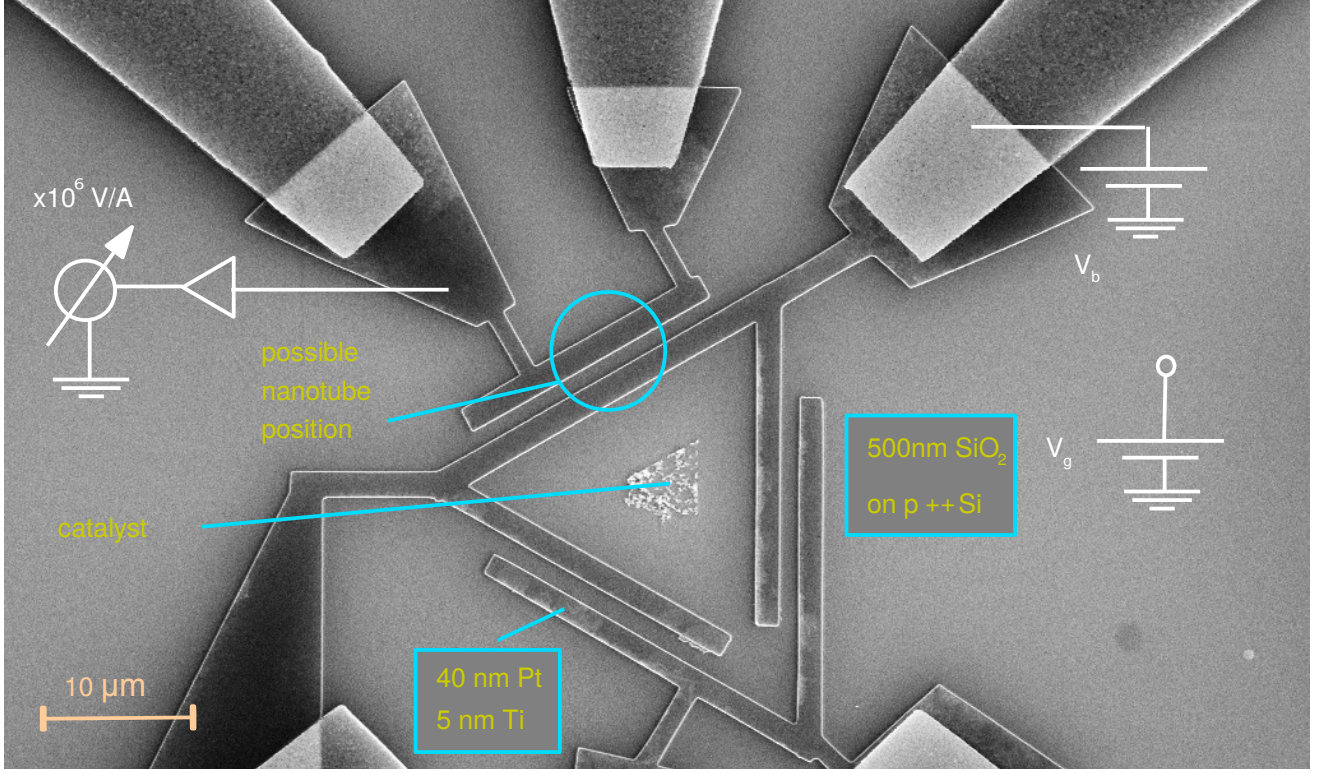

FIG. S1. Electron micrograph of a chip similar to the measured device. The Pt/Ti structures on top of the Si/SiO<sub>2</sub> are clearly visible. In the center of the triangular structure a residual of the catalyst can be found. Schematic drawings indicate the measurement circuit.

The average length of the electron path in the interferometer can be calculated by considering the probability to perform  $n$  laps,  $P_n = (|r_1|^2|r_2|^2)^n$ , multiplied by the path length  $2nL$ , i.e.,

$$l_{\text{avg}} = L + |r_1|^2|r_2|^2 2L + \dots + (|r_1|^2|r_2|^2)^n 2nL + \dots = \left[ 1 + \frac{2|r_1|^2|r_2|^2}{(1 - |r_1|^2|r_2|^2)^2} \right] L, \quad (\text{S2})$$

where the first term reflects the directly transmitted electron. To calculate the Fourier coefficients we note that  $T(k_j)$  in Eq. (S1) is even and  $\pi/L$ -periodic as a function of  $k_j$ . Therefore it can be expanded in a Fourier series,

$$T(k) = \sum_n \alpha_n \cos(2nkL),$$

with the Fourier coefficients

$$\alpha_n = \frac{L}{\pi} \int_{-\pi/2L}^{\pi/2L} T(k) \cos(2nkL) dk.$$

While the calculation of the coefficients in general is cumbersome, it can be shown that the ratio of two coefficients yields the product of the two reflection coefficients, i.e.,<sup>2</sup>

$$\frac{\alpha_{n+1}}{\alpha_n} = |r_1||r_2|.$$

The coefficients can thus be written as

$$\alpha_n = \alpha_0 (|r_1||r_2|)^n, \quad (\text{S3})$$

where  $m = n + 1$  is the harmonic order, i.e.,  $mf_1 = f_m$ . Fig. S2 shows fits of Eq. (S3) to the amplitudes of the Fourier transform (Fig. 1(d) of the main text). Note that the amplitudes of the harmonics in the FT are oscillating

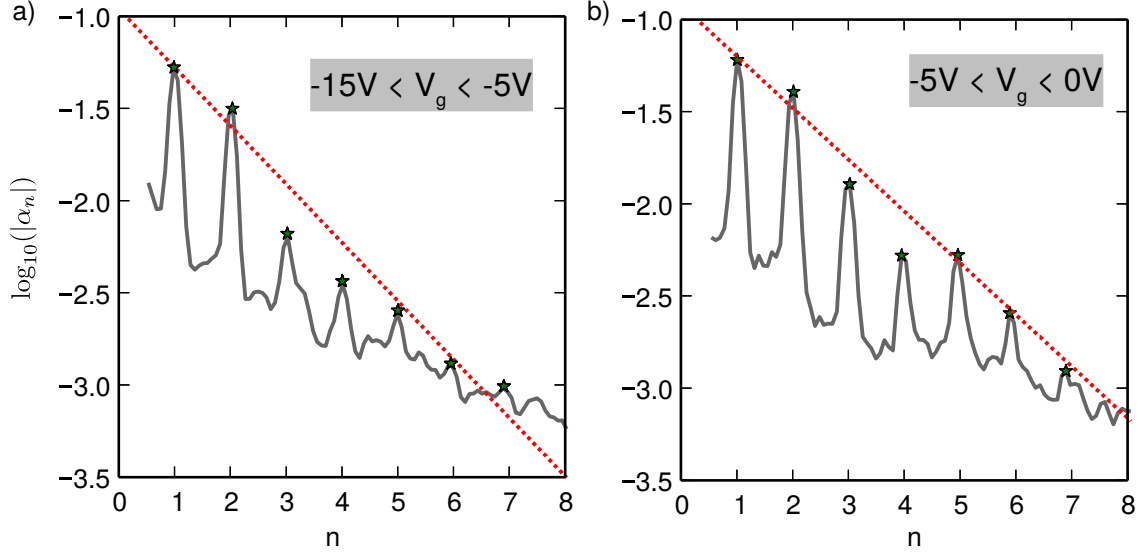

FIG. S2. Amplitude decay of the amplitudes of the frequency components in the Fourier transform shown in Fig. 1(d) of the main text. The graphs are displayed on a logarithmic scale.  $n$  is the harmonic order with  $nf_1$  being the frequency of the  $n$ -th harmonic component. The stars denote peak positions that are used for the fit to Eq. (S3) (dashed line). (a) Amplitudes averaged over a gate voltage range of  $-15\text{ V} < V_g < -5\text{ V}$ . (b) Amplitudes averaged over a gate voltage range of  $-5\text{ V} < V_g < 0\text{ V}$ .

when we change the gate voltage, see Fig. 1(d). Since this is not accounted for in Eq. (S3), we have to average the FT amplitude over a gate voltage range that includes multiple periods of the slow modulation to compare the FT data to Eq. (S3). To this end, we divide the full gate voltage range into two ranges,  $[-15\text{ V}, -5\text{ V}]$  and  $[-5\text{ V}, 0\text{ V}]$ . The average of the FT amplitudes for the two ranges is shown in Fig. S2(a,b), respectively, as a function of  $n$ . We fit Eq. (S3) to the curve and extract the product  $|r_1||r_2|$  of the reflection coefficients. This product can be used in Eq. (S2) to obtain the average electronic path length. We obtain  $l_1 = 2.6L$  and  $l_2 = 3.3L$  for the  $[-15\text{ V}, -5\text{ V}]$  and the  $[-5\text{ V}, 0\text{ V}]$  gate voltage range, respectively.

### III. TRANSFER MATRIX APPROACH

Using a simple (non-unitary) transfer matrix description of the system,<sup>3</sup> we can understand the evolution of the slow modulation of the conductance in armchair-like CNTs from the mixing of the channels upon reflection at the contacts. We consider two waves in the channels  $a$  and  $b$  before and after the scattering event. For simplicity, we consider only one pair of incident waves from one side of the cavity and one pair of outgoing waves on the other side of the cavity. Since we do not study the full scattering problem, which would include both in- and out-going waves on both sides of the cavity, the amplitudes can not be related to probabilities. The initial and final states are represented by the vectors

$$|i\rangle = \begin{pmatrix} a \\ b \end{pmatrix} \quad (\text{initial}) \quad \text{and} \quad |f\rangle = \mathbf{M}|i\rangle \quad (\text{final}),$$

where  $\mathbf{M}$  is a (complex) two-by-two transfer matrix and  $a$  and  $b$  are complex numbers characterizing the plane waves before entering the cavity. Although  $\mathbf{M}$  is not describing the full scattering problem, the squares of the amplitude of the transmitted wave  $|f\rangle$  in the two channels reproduce the transmission  $\mathcal{T}$ , i.e.,

$$\mathcal{T} \propto \sum_{ij} |\mathbf{M}_{ij}|^2. \quad (\text{S4})$$

$\mathbf{M}$  is constructed from a product of matrices which describe the effect of different elements of the cavity on the wave function. In particular, the transmission through the (symmetric) left and right barriers is described by matrices

$$\mathbf{T} = \mathbf{T}_l = \mathbf{T}_r = \begin{pmatrix} t & 0 \\ 0 & t \end{pmatrix}.$$

where the coefficients  $t$  are real for simplicity. Passing through the CNT we acquire gate voltage dependent phases  $\phi_a(V_g)$  and  $\phi_b(V_g)$  in the two modes, respectively:

$$\mathbf{T}_c = \begin{pmatrix} e^{i\phi_a} & 0 \\ 0 & e^{i\phi_b} \end{pmatrix}.$$

The reflection at the two interfaces is described by

$$\mathbf{R} = \mathbf{R}_l = \mathbf{R}_r = \begin{pmatrix} r & r' \\ r' & r \end{pmatrix},$$

where  $r'$  induces a *mixing* of the channels.

We calculate  $\mathbf{M}$  taking into account two different electron paths in the cavity. This is the minimal ingredient to observe wave interference in the transmitted signal. The first electronic path is one where the electron is directly transmitted, while in the second path it travels one extra lap before leaving the cavity. The transfer matrix reads

$$\mathbf{M} = \mathbf{T}\mathbf{T}_c\mathbf{T} + \mathbf{T}\mathbf{T}_c\mathbf{R}\mathbf{T}_c\mathbf{R}\mathbf{T}_c\mathbf{T} = \mathbf{T}\mathbf{T}_c(\mathbb{1} + \mathbf{R}\mathbf{T}_c\mathbf{R}\mathbf{T}_c)\mathbf{T}. \quad (\text{S5})$$

When we relate  $\mathbf{M}$  to the transmission using Eq. (S4), the matrices  $\mathbf{T}\mathbf{T}_c$  and  $\mathbf{T}$  outside the bracket only add global phases and amplitudes to the diagonal elements. The global phases vanish when taking the absolute values and the global amplitudes are not important for our argument. Evaluating the part in brackets in Eq. (S5), we obtain

$$\mathbb{1} + \mathbf{R}\mathbf{T}_c\mathbf{R}\mathbf{T}_c = \begin{pmatrix} 1 + r^2 e^{2i\phi_a} + r'^2 e^{i(\phi_a + \phi_b)} & rr' (e^{i(\phi_a + \phi_b)} + e^{i2\phi_b}) \\ rr' (e^{i(\phi_a + \phi_b)} + e^{i2\phi_a}) & 1 + r^2 e^{2i\phi_b} + r'^2 e^{i(\phi_a + \phi_b)} \end{pmatrix}. \quad (\text{S6})$$

In the pure armchair case  $r' = 0$ , so we end up with a diagonal matrix and obtain, using Eq. (S4),

$$\mathcal{T} \propto \sum_{n=1}^2 |\mathbb{1} + \mathbf{R}\mathbf{T}_c\mathbf{R}\mathbf{T}_c|_{nn}|^2 = 2 \{1 + r^4 + r^2 [\cos(2\phi_a) + \cos(2\phi_b)]\}, \quad (\text{S7})$$

where  $[M]_{ij}$  refers to the matrix element  $M_{ij}$ . The transmission can be identified as a beat of two waves with phases  $\phi_a \neq \phi_b$  as a function of the gate voltage.

When we allow for  $r' \neq 0$ , the square of the absolute values of a diagonal entry of the matrix in Eq. (S6),

$$|\mathbb{1} + \mathbf{R}\mathbf{T}_c\mathbf{R}\mathbf{T}_c|_{11}|^2 = 1 + r^4 + 2r^2 \cos(2\phi_a) + 2r'^2 \cos(\phi_a + \phi_b) + 2r^2 r'^2 \cos(\phi_a - \phi_b) + \mathcal{O}(r'^4), \quad (\text{S8})$$

is proportional to the cosine of the phase difference  $\phi_a - \phi_b$ . Note that the off-diagonal entries,

$$|\mathbb{1} + \mathbf{R}\mathbf{T}_c\mathbf{R}\mathbf{T}_c|_{12}|^2 = [\mathbb{1} + \mathbf{R}\mathbf{T}_c\mathbf{R}\mathbf{T}_c]_{21} = 2r^2 r'^2 (1 + \cos(\phi_a - \phi_b)), \quad (\text{S9})$$

contain these phase differences, too. They are responsible for the slow oscillation of the conductance and its sliding average.

In Fig. S3 we plot  $\sum_{ij} |\mathbf{M}_{ij}|^2$  as a function of energy for different values of  $r'$ . To obtain the plots, we write the function  $\phi_j(E)$  as a second order polynomial with a slightly different coefficient in front of the quadratic term for the two channels  $j$ . This reflects a different dispersion relation of the two channels. In Fig. S3(a), the mixing is absent,  $r' = 0$ , and Eq. (S7) shows a beat. The hull curve evolves with a phase  $\phi_a - \phi_b$ , see Fig. S3(a), exhibiting two maxima of transmission within one period. The average of the transmission calculated over a few periods of  $\phi_a$  or  $\phi_b$  is constant since both constituents of the transmission function bear a constant average. In (b), the finite mixing  $r'$  leads to a deformation of every second anti-node (i.e., regions with constructive interference). The sliding average (green line in (b)) is slightly modulated. The even stronger channel mixing in Fig. S3(c) induces a more prominent modulation of the transmission as a function of the phase difference. Finally, in Fig. S3(d) via complex values of  $r'_{R/L}$  a phase shift of the wavefunction upon reflection at the barriers is introduced. This leads to additional regions of apparent frequency doubling which occur next to the maxima of the sliding conductance average, similar to the measurement data of Fig. 1(b) in the main manuscript.

#### IV. TIGHT-BINDING CALCULATIONS

For our numerical calculations we use a tight-binding Hamiltonian for the description of the CNT. We consider interactions up to first-nearest neighbors and we restrict ourselves to one  $2p$  orbital per atom. The  $2p$  orbitals give rise

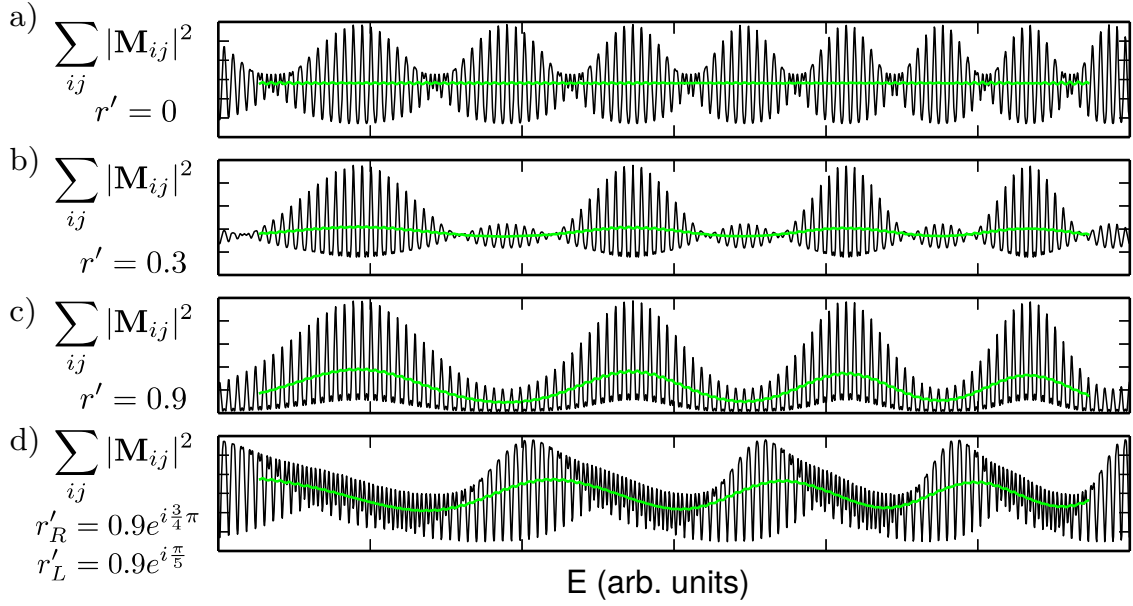

FIG. S3. The sum  $\sum_{ij} |M_{ij}|^2$  plotted as a function of energy in arbitrary units. The green line is the sliding average of the black line.  $\phi_a(E)$  and  $\phi_b(E)$  are given by second order polynomials with slightly different quadratic prefactor. (a)  $r' = 0$ , no mode mixing occurs and a beat can be observed. The sliding average is constant. (b,c) Mode mixing is increased to  $r' = 0.3$  (b) and to  $r' = 0.9$  (c). The off-diagonal terms induce a slow modulation of the signal that is reflected also in the sliding average. (d) In addition, phase shifts of the wavefunction upon reflection at the contacts are introduced. While the slow modulation of the sliding average remains present, additionally regions of apparent frequency doubling appear.

to the  $\pi$  and  $\pi^*$  bands, which are responsible for the CNT's conduction as the next molecular orbitals lie energetically far apart.

The Hamiltonian describing our systems reads

$$H_0 = \sum_i \epsilon_{2p} c_i^\dagger c_i + \sum_{\langle i,j \rangle, i \neq j} t_{ij} c_i^\dagger c_j, \quad (\text{S10})$$

where the indices  $\langle i, j \rangle$  indicate nearest neighbor atom sites and the summation is extended over all the points in the lattice. The transfer integrals  $\epsilon_{2p}$  are the onsite energies and  $t_{ij}$  are the hopping parameters. Our energy scale is shifted in order to have vanishing on-site energies, setting  $\epsilon_{2p} = 0$ . For the hopping parameter  $t_{ij}$  we choose  $t = -2.66$  eV, as we used the Tománek-Louie parametrization for graphite up to nearest-neighbor interactions.<sup>4</sup> This parametrization includes also the  $\sigma$  molecular orbitals, and has been proven to be a consistent parameter set. The  $\sigma$  orbitals mix with the  $\pi$  molecular orbitals due to the finite curvature. Therefore, to take into account curvature and include also spin-orbit effects in our calculations, we need a set of parameters containing the Slater-Koster transfer integrals for the different molecular orbitals. The transfer integrals describing the hopping between nearest neighbors are not given by constants any more but depend on the relative three-dimensional position of the atoms, and on the strength of the spin-orbit interaction. The derivation of these transfer integrals can be found in Ref. 5, together with the spin-orbit coupling parameter used in our numerical calculations. The finite curvature and spin-orbit interaction do not affect the main secondary interference pattern in our numerical results. For simplicity, calculations in the main text do not include these effects.

The barriers at the interfaces with the leads are modelled by considering a reduced hopping parameter  $t_{ij}^c = 0.73t_{ij}$  and an enlarged onsite energy  $\epsilon_{2p} = 0.07$  eV for the atoms on the ring that forms the contact to the leads. This model of the barriers has been used successfully in real-space transport calculations in the Fabry-Perot regime.<sup>6</sup> In the numerical results shown in the main text, all on-site energies on the contact ring are equal. Thus, the barriers respect the symmetries (rotational, parity) of all CNTs. We consider semi-infinite CNTs as leads to model transparent contacts. Additional numerical calculations where the hopping parameter and the onsite energy are not only modified on a narrow ring of atoms, but for an extended contact region, have also been performed and display very similar interference behavior; see Fig. S7 for an example.

When we consider CNTs with lengths in the range of  $\mu\text{m}$ , we need to reduce computational costs by simplifying the Hamiltonian describing the CNT through the application of decimation techniques.<sup>7</sup> For the computation of the

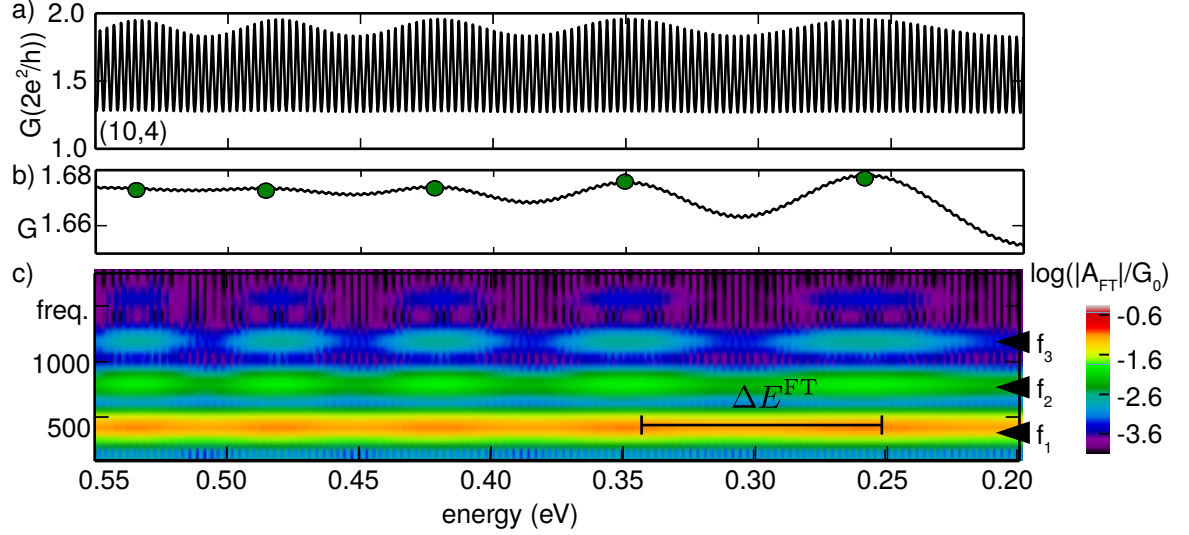

FIG. S4. (a) Transmission of an armchair-like (10,4) CNT ( $L = 660$  nm) from tight-binding calculations including curvature and spin-orbit effects. The secondary interference pattern, i.e., a modulation of the conductance over a period of  $0.05 - 0.10$  eV, is evident. (b) Average value of (a) obtained using a  $0.019$  eV-wide sliding window. Slow oscillations of the average conductance values are clearly visible. The peak positions are marked by filled circles. (c) Fourier transform of the transmission signals in (a) using a  $0.019$  eV window function. The amplitudes of the higher harmonic components vary in phase with the fundamental frequency component with a period  $\Delta E^{\text{FT}}$ .

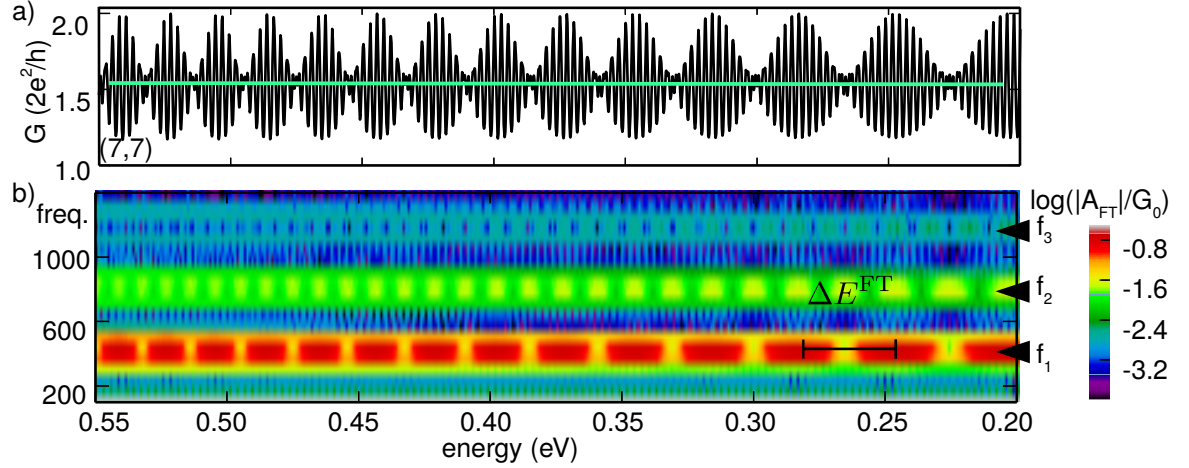

FIG. S5. (a) Transmission of a (7,7) armchair CNT ( $L = 660$  nm) from tight-binding calculations including curvature and spin-orbit effects. The average is constant (green line). (b) Fourier transform of (a) using a sliding  $0.015$  eV window function. The amplitudes of the frequency component of harmonic order  $n$  vary with a period  $\Delta E^{\text{FT}}/n$ .

coherent transport in these systems, the conductance is calculated within the Landauer approach. We therefore use the Green's functions constructed from the real-space Hamiltonians and then make use of the Fisher-Lee relation for the computation of the conductance.<sup>8</sup>

In Fig. S4(a) we show the results for the transmission of a (10,4) armchair-like CNT with a length  $L = 660$  nm. The secondary interference pattern can be observed. The sliding average of the transmission in (b) follows the slow modulation of the transmission signal. In contrast, the transmission through the (7,7) armchair nanotube in Fig. S5(a) exhibits a beat, and the sliding average (green line) is constant.

The differences between the two geometries manifest themselves also in the Fourier transforms. In the Fourier transform of the armchair-like CNT in Fig. S4(c) we observe an oscillation of the amplitudes of the different frequency components  $f_n$  with energy. This period, labelled by  $\Delta E^{\text{FT}}$  in the plot, is the same for all orders  $n$ . On the other

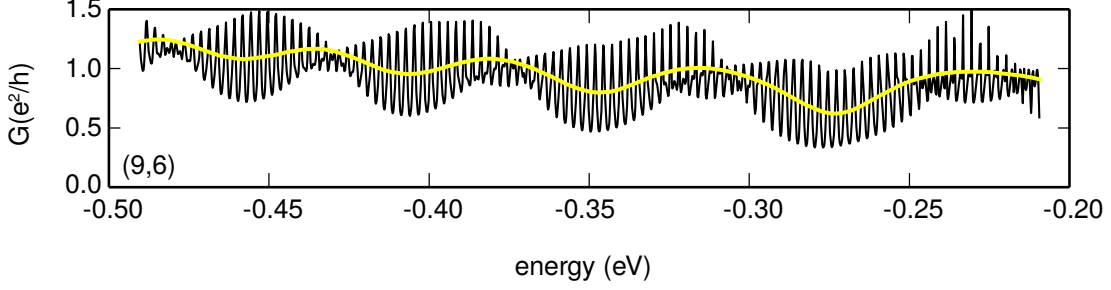

FIG. S6. Influence of extrinsic symmetry breaking at the contacts. The conductance of a zigzag-like (9,6) CNT ( $L = 660$  nm) is calculated with no curvature or spin-orbit effects. An asymmetric distribution of on-site energies  $\epsilon_{2p}$  on the contact ring is used, with values of  $\epsilon_{2p} = 5$  eV at the top and  $\epsilon_{2p} = 1$  eV at the bottom. The secondary interference pattern is clearly seen.

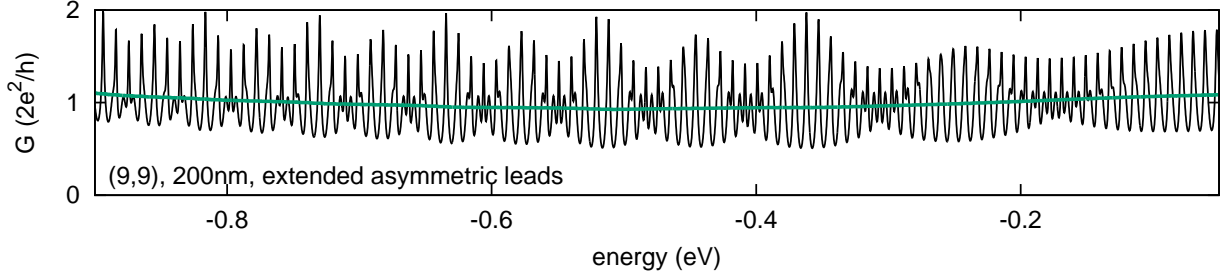

FIG. S7. Tight-binding calculation of the conductance for an armchair (9,9) CNT ( $L = 200$  nm). The on-site energies  $\epsilon_{2p}$  are asymmetrically modified over extended contact regions, with values of  $\epsilon_{2p} = 5$  eV at the top and  $\epsilon_{2p} = 1$  eV at the bottom of the CNT. No slow modulation of the conductance is observed, since parity symmetry still prevents channel mixing.

hand, in the Fourier transform of the armchair nanotube, Fig. S5(b), the amplitude of the  $n$ -th harmonic oscillates with a period  $\Delta E^{\text{FT}}/n$ .

### Symmetry-breaking in the leads

The numerical calculations show that the secondary interference patterns in the Fabry-Perot transport regime depend on the symmetries of the CNT *including* their contact regions. That is, when parity symmetry is preserved in the presence of contacts in *armchair* CNT based waveguides, a beat pattern as in Fig. S5 will be seen. *Zigzag-like* CNT waveguides will show the behavior corresponding to a single channel when the rotational symmetry is preserved by the contacts, as explained in the main text.

We have tested numerically the robustness of the Fabry-Perot patterns against a breaking of the rotational symmetry in the contact region of *zigzag-like* CNTs. The contact regions at both ends are modeled as a ring of atoms terminating the CNT. In the following, we break the rotational symmetry of the system by choosing largely different on-site energies on the bottom half of the ring,  $\epsilon_{2p} = 1$  eV, and on the top half of the ring,  $\epsilon_{2p} = 5$  eV. In this way we model the electric contact to the metallic leads that support the otherwise suspended CNT.

In Fig. S6 we show the calculated conductance for a *zigzag-like* (9,6) CNT. We observe a clear deviation from the single-channel behavior, and a secondary interference pattern including a modulation of the sliding average  $\bar{G}(V_g)$  (yellow line in Fig. S6). The slow modulation can be understood from the mixing of the transport channels induced by the contact asymmetry. This effect is similar to what we observe for *armchair-like* CNTs. While the mixing is an intrinsic effect in *armchair-like* CNTs due to the absence of symmetries preventing it, the extrinsic breaking of the rotational symmetry is required to induce it also in *zigzag-like* CNTs.

Achiral *zigzag* CNTs are not sensitive to symmetry-breaking in the leads. In this case, the induced channel mixing has no effect because electrons in both channels accumulate the same phase.<sup>9</sup> Consequently, the sliding average does not oscillate over the gate voltage range. Similarly, for *armchair* CNTs we do not find a modulation of the sliding average in the presence of asymmetric contacts; see Fig. S7 for a corresponding calculation where extended contact regions of broken rotational symmetry are used.

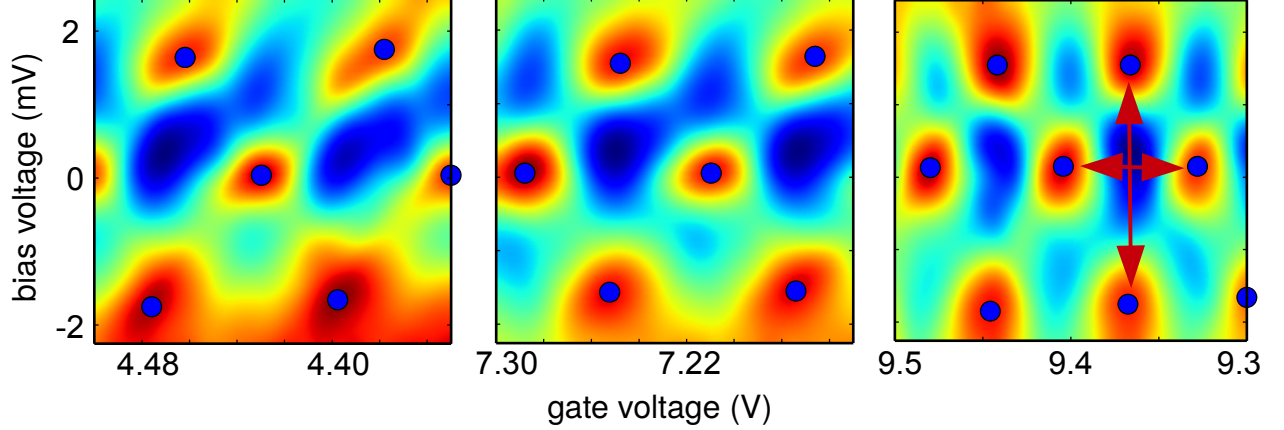

FIG. S8.  $G(V_g, V_b)$  in three regions of constructive interference. The experimental data is smoothened. Filled blue circles mark the positions of maxima that are used to evaluate  $\alpha$ . In the rightmost panel, arrows indicate the distances  $\Delta V_b$  and  $\Delta V_g$ , respectively.

### Frequency doubling behavior

One of the characteristic effects accompanying the slow modulation of the conductance is an apparent frequency doubling of  $G(V_g)$  within distinct gate voltage regions of each modulation period, see Fig. 1 of the main manuscript. These corresponding regions are those where the first harmonic dominates over the fundamental frequency in the Fourier transform of  $G(V_g)$ , cf. Fig. 1(b) and Fig. 1(d).

A comparison with the results of the tight-binding calculations shows distinct differences. As examples, for the *armchair-like* (10,4) CNT, see Fig. S4, the maxima of the harmonics occur at the same energies as those of the fundamental frequency, i.e., the fundamental frequency remains always dominant and no apparent frequency doubling can be seen. For the *armchair* (7,7) CNT of Fig. S5, even though the average conductance is constant, the harmonics display different periodicity in  $V_g$  compared to the fundamental, leading to small intervals of apparent frequency doubling whenever the fundamental is weakest. Finally, for the *zigzag-like* (9,6) CNT with extrinsic symmetry breaking, see Fig. S6, very similar to the measurement, regular regions of apparent frequency doubling next to the maxima of the averaged conductance  $\bar{G}(V_g)$  occur.

The precise interplay of the apparent frequency doubling with chiral class, chiral angle and boundary conditions still has to be determined and goes beyond the scope of this work. As seen from Fig. S6, also microscopic details of the contact regions enter here. A comparison with the transfer-matrix calculation of Fig. S3(d) suggests that one consequence of the rotational symmetry breaking in the contacts might be the introduction of different reflection phases. In any case, the slow modulation of the average conductance as discussed in the main manuscript allows a more universal and robust evaluation.

### V. ESTIMATE OF THE ERROR IN DETERMINING THE CHIRAL ANGLE

In the Fig. 3 of the main text, error bars indicate a range of acceptable values for the chiral angle  $\theta$ . This is the result of an analysis of the three different sources of uncertainty in the evaluation. Those are: the uncertainty in the distance between  $V_g = 0$  V and the center of the bandgap,  $\Delta E_{\text{gap}}$ , the uncertainty in the gate voltage lever arm  $\alpha$  and in the overlap integral used in the tight-binding model,  $t = 2.6 \pm 0.1$  eV.<sup>10</sup> We introduce the sources of the uncertainty in the fit and present  $P$ -value maps of the parameter space.

*a. The gate voltage lever arm in the hole region* We extract the lever arm  $\alpha$  in the hole region, i.e., for  $V_g < 1$  V, by analyzing the FP pattern in the conductance,  $G(V_g, V_b)$ , Fig. 1(a) of the main text, in three regions with high conductance, shown in Fig. S8. We assume that in these regions constructive interference leads to a single channel interference pattern which allows the extraction of the lever arm in accordance with Liang *et al.*<sup>11</sup> The filled circles in Fig. S8 highlight the peak positions that are used to determine the gate voltage lever arm,  $\alpha = \Delta V_b / 2\Delta V_g$ , where  $\Delta V_b$  and  $\Delta V_g$  denote the differences in bias and gate voltage between two peaks, respectively. These distances are highlighted by arrows in Fig. S8(c). From these distances we evaluate  $\alpha = 0.0210 \pm 0.0007$ .

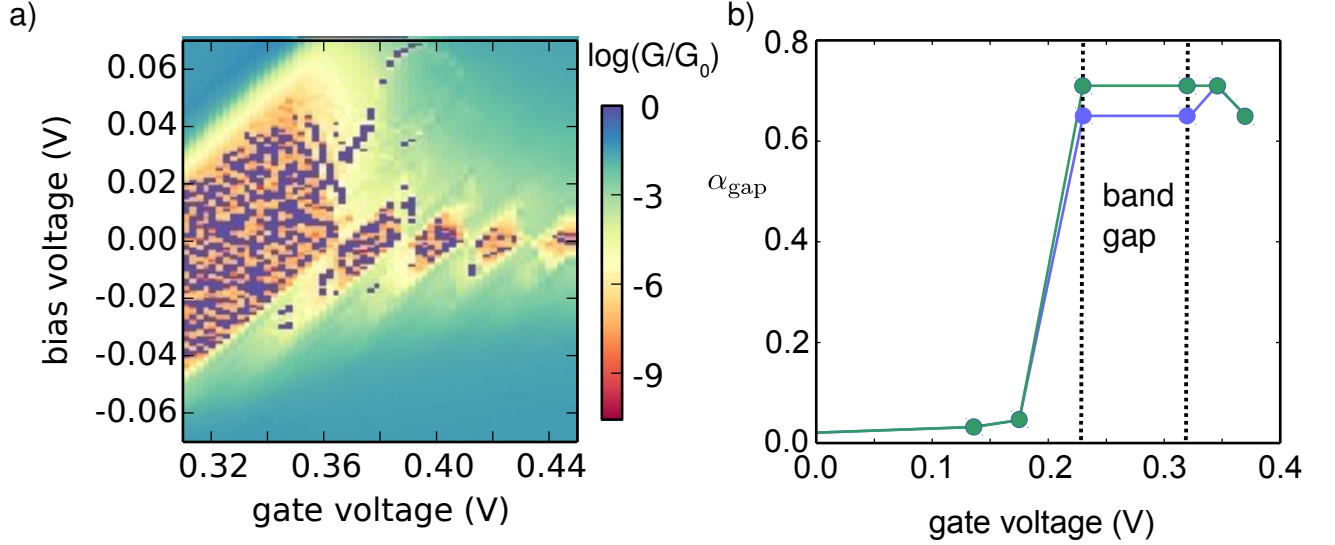

FIG. S9. (a)  $\log(G(V_b, V_g)/G_0)$  in the bandgap region and for the first few electron states. The left upper edge (source line) of the bandgap is clearly visible, while the right upper edge (drain line) is not clearly resolved and induces an error in the determination of the lever arm in the bandgap and, similarly, the height of the bandgap. The gate voltage axis in this measurement is shifted slightly with respect to the data in Fig. 1 of the main text. (b)  $\alpha_{\text{gap}}$  in the vicinity of the bandgap. The two lines represent the bounds for  $\alpha_{\text{gap}}$  in the bandgap region.

Notably, the frequency  $f_1 \simeq 12.8 \frac{1}{V}$  of the fundamental component in the Fourier map in Fig. 1(d) of the main text is constant over the whole range up to  $V_g = -1$  V. If the lever arm changed with gate voltage in this range,  $f_1$  would be affected by this change as well. We can therefore assume that the gate voltage lever arm stays approximately constant in the range  $-15 \text{ V} < V_g < -1$  V.

*b. The bandgap offset* When we want to compare the evolution of the phase difference  $\Delta\phi^\theta(E)$  (obtained from the tight-binding dispersion relation) with the experimental data, we have to measure  $E$  from a unique, distinguishable point, i.e., the Dirac point where conductance and valence band touch in the theoretical model. In the experimental data, we identify the center of the small bandgap at  $V_g = 0.28$  V with the Dirac point.<sup>12</sup> Therefore we have to shift the experimental points by an energy  $\Delta E_{\text{gap}} = \int_{0 \text{ V}}^{0.28 \text{ V}} \alpha_{\text{gap}}(V_g) dV_g$ . The difficulty in measuring this distance is given by the variation of the lever arm  $\alpha_{\text{gap}}(V_g)$  in the vicinity of the bandgap. In Fig. S9(a), the conductance in the vicinity of the bandgap and the first electronic charging states are shown. From the data, the gate voltage lever arm within the bandgap can be extracted with 10% accuracy, see Fig. S9(b). The bounds for this value are indicated by the two lines. The total shift of the values  $E_n$  is given by the area under each line in Fig. S9(b) yielding a range  $\Delta E_{\text{gap}} = 0.60 \pm 0.05$  eV.

*c. The tight-binding overlap integral* We fit the experimental data points using the inverse of the CNT tight-binding dispersion relation  $k_{j,i}^\theta(E) = [\varepsilon(k_{j,i}^\theta)]^{-1}$ . The overlap integral  $t$  between electrons occupying neighboring sites in the tight-binding model,  $t$ , determines the slope of the dispersion relation and is tightly connected to the electron group velocity  $v_F = \partial E / \hbar \partial k = \sqrt{3}at/2$ . For the overlap integral, a value of  $t = 2.5$  eV is found to describe the graphene dispersion from theoretical grounds,<sup>10</sup> corresponding to a Fermi velocity of  $v_F \approx 8 \cdot 10^5$  m/s. Experimentally, a value of  $t = 2.6$  eV is found from the analysis of bandgaps in metallic zigzag CNTs<sup>13</sup> and  $t = 2.7$  eV has been used to fit CNT bandgaps as a function of the radius in chiral nanotubes.<sup>14</sup> This value corresponds to a Fermi velocity of  $v_F \approx 9 \cdot 10^5$  m/s.

### The quality of the fit

The model dispersion is determined by the chiral angle  $\theta$ , the offset  $\Delta E_{\text{gap}}$  and the overlap integral  $t$ . For each set of parameters we calculate the  $\chi^2$  value,

$$\chi^2(\theta, \Delta E_{\text{gap}}, t) = \sum_n \frac{1}{\sigma_n^2} [E(n, \theta, t) - (E_n + \Delta E_{\text{gap}})]^2,$$

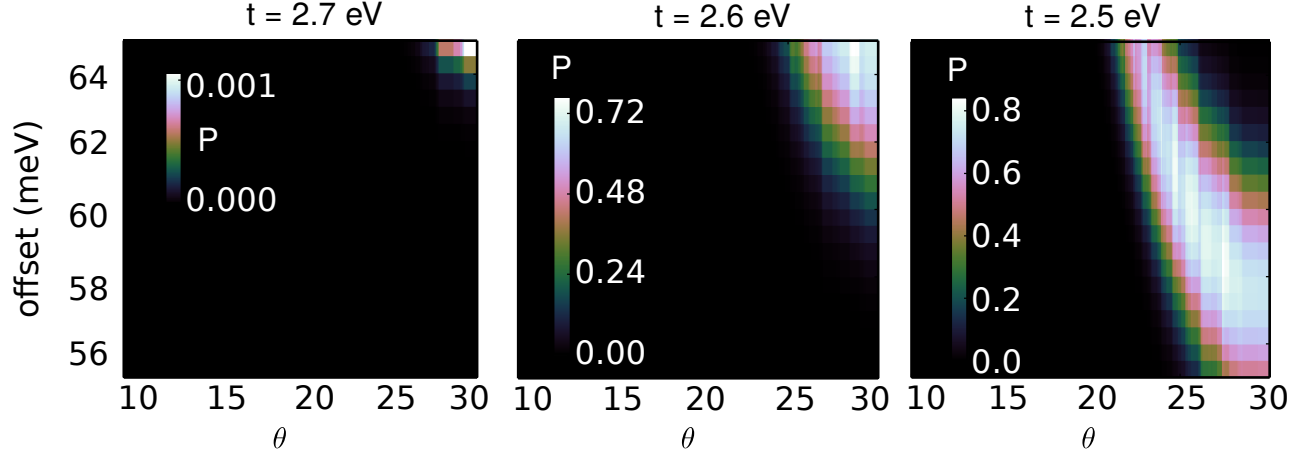

FIG. S10.  $P(\theta, \Delta E_{\text{gap}})$  for different values of  $t$ . Note that the range of the color bar in the first panel is smaller by two orders of magnitude compared to the other two. A value of  $t = 2.7$  eV is not consistent with our data.

where the values  $E(n, \theta, t)$  are obtained from the condition  $\Delta\phi^\theta(E, t) \stackrel{!}{=} 2\pi n$  and  $\sigma_n$  is the error in the estimation of the peak positions  $E_n$ , which is mainly determined by the error of  $\alpha$  for  $V_g < -2$  V. From the  $\chi^2$  value we calculate the  $P$ -value,  $P = 1 - F_\nu(\chi^2)$ , where  $F_\nu$  is the cumulative distribution function for the  $\chi^2$  distribution,  $\nu = N - N_p$  is the number of degrees of freedom,  $N = 7$  is the number of points for the fit and  $N_p = 2$  is the number of free parameters.<sup>15</sup> Thereby, apart from the chiral angle  $\theta$ , the bandgap offset  $\Delta E_{\text{gap}}$  is taken as a free parameter which is allowed to vary within the bounds estimated above. In Fig. S10 we show  $P(\theta, \Delta E_{\text{gap}})$  for different values of the overlap integral in the tight-binding dispersion relation,  $t$ . By setting a threshold value of  $P < 0.05$  for rejecting the fit, we find that a value of  $t = 2.7$  eV is not consistent with our data, while  $2.5 \text{ eV} \leq t \leq 2.6 \text{ eV}$  is consistent, see the left panel in Fig. S10. In addition, the acceptable values for the chiral angle lie in the range  $22^\circ < \theta < 30^\circ$ .

---

\* andreas.huettel@ur.de

- <sup>1</sup> A. K. Hüttel, G. A. Steele, B. Witkamp, M. Poot, L. P. Kouwenhoven, and H. S. J. van der Zant, Nano Letters **9**, 2547 (2009).
- <sup>2</sup> D. Hofstetter and R. L. Thornton, Opt. Lett. **22**, 1831 (1997).
- <sup>3</sup> M. Born, *Principles of optics electromagnetic theory of propagation, interference, and diffraction of light*. (Pergamon Press, Oxford; New York, 1964).
- <sup>4</sup> D. Tománek and S. G. Louie, Physical Review B **37**, 8327 (1988).
- <sup>5</sup> M. del Valle, M. Margańska, and M. Grifoni, Phys. Rev. B **84**, 165427 (2011).
- <sup>6</sup> S. Krompiewski, J. Martinek, and J. Barnaś, Phys. Rev. B **66**, 073412 (2002).
- <sup>7</sup> C. J. Lambert and D. Weaire, physica status solidi (b) **101**, 591 (1980).
- <sup>8</sup> S. Datta, *Electronic transport in mesoscopic systems* (Cambridge University Press, 1997) p. 377.
- <sup>9</sup> J. Jiang, J. Dong, and D. Xing, Phys. Rev. Lett. **91**, 056802 (2003).
- <sup>10</sup> R. Saito, M. Dresselhaus, and G. Dresselhaus, *Physical Properties Of Carbon Nanotubes* (World Scientific, 1998).
- <sup>11</sup> W. Liang, M. Bockrath, D. Bozovic, J. H. Hafner, M. Tinkham, and H. Park, Nature **411**, 665 (2001).
- <sup>12</sup> The simple (nearest-neighbor) model does not account for the experimentally observed small bandgap. However, this does not effect our analysis of the interference pattern deep in the hole regime ( $V_g < -2$  V). The analysis in this range is not affected by the deformation of the conduction band in the direct vicinity of the band gap.
- <sup>13</sup> M. Ouyang, J. L. Huang, C. L. Cheung, and C. M. Lieber, Science (New York, N.Y.) **292**, 702 (2001).
- <sup>14</sup> J. W. G. Wildoer, L. C. Venema, A. G. Rinzler, R. E. Smalley, and C. Dekker, Nature **391**, 59 (1998).
- <sup>15</sup> J. R. Taylor, *An Introduction to Error Analysis: The Study of Uncertainties in Physical Measurements* (1997).
